# Supplementary material for: On the irreducible character degrees of symmetric groups and their multiplicities
Source: arXiv:2410.01726 ancillary file (2025-04-23)
Supplement: Supplementary file 1 [file symmetric.pdf]

# Magma Package **symmetric**

David A. Craven

Version 1.3: March 27, 2025

# Contents

|          |                                                       |           |
|----------|-------------------------------------------------------|-----------|
| <b>1</b> | <b>Functions regarding partitions</b>                 | <b>2</b>  |
| 1.1      | Printing partitions . . . . .                         | 2         |
| 1.2      | Counting partitions . . . . .                         | 2         |
| 1.3      | Special partitions . . . . .                          | 2         |
| 1.4      | Self-conjugate partitions . . . . .                   | 3         |
| 1.5      | Iterator for partitions . . . . .                     | 3         |
| 1.6      | Hooks, $\beta$ -sets, etc. . . . .                    | 4         |
| 1.7      | Conjugacy classes . . . . .                           | 5         |
| <b>2</b> | <b>Character degrees and their multiplicities</b>     | <b>6</b>  |
| 2.1      | Maximal character degrees . . . . .                   | 6         |
| 2.2      | Multiplicities of character degrees . . . . .         | 7         |
| 2.3      | $\infty$ -partitions and partition clusters . . . . . | 7         |
| 2.3.1    | General commands . . . . .                            | 7         |
| 2.3.2    | Commands to access databases . . . . .                | 9         |
| 2.4      | Characters for $GL_n(q)$ and $GU_n(q)$ . . . . .      | 9         |
| <b>3</b> | <b>Restrictions of characters of Sylow subgroups</b>  | <b>11</b> |
| <b>4</b> | <b>Changes since original</b>                         | <b>13</b> |

The aim of this documentation is to cover all of the new commands introduced in the `symmetric` package.  
To run it, use `AttachSpec("symmetric.s");`.

# Chapter 1

## Functions regarding partitions

### 1.1 Printing partitions

`PrintReducedFormPartition(pa::SeqEnum[RngIntElt]) -> MonStgElt`

Prints a partition in reduced form, suitable to including in a  $\text{\LaTeX}$  document. So, for example, the partition with one 3 and nine 1s is printed as  $(3, 1^9)$ .

### 1.2 Counting partitions

`NumberOfPartitionsWithAtMostParts(n::RngIntElt, k::RngIntElt) -> RngIntElt`

Given a non-negative integer  $n$  and a positive integer  $k$ , returns the number of partitions of  $n$  into at most  $k$  parts.

`NumberOfPartitionsWithExactlyParts(n::RngIntElt, k::RngIntElt) -> RngIntElt`

Given a non-negative integer  $n$  and a positive integer  $k$ , returns the number of partitions of  $n$  into exactly  $k$  parts.

### 1.3 Special partitions

`HookPartitions(n::RngIntElt) -> SeqEnum`

The collection of all hook partitions of size  $n$ , ordered lexicographically.

`AlmostHookPartitions(n::RngIntElt) -> SeqEnum`

The collection of all almost-hook partitions of size  $n$ , ordered lexicographically.

`TwoPartPartitions(n::RngIntElt) -> SeqEnum`

The collection of all partitions of size  $n$  with exactly two parts, ordered lexicographically.

`ThreePartPartitions(n::RngIntElt) -> SeqEnum`

The collection of all partitions of size  $n$  with exactly three parts, ordered lexicographically.

## 1.4 Self-conjugate partitions

`IsSelfConjugate(pa::SeqEnum[RngIntElt]) -> BoolElt`

Return true if the partition `pa` is self-conjugate. Input must be a partition with no trailing zeros.

`SelfConjugatePartitions(n::RngIntElt,k::RngIntElt) -> SeqEnum`

The self-conjugate partitions of `n` of length at most `k` (or equivalently with first row of size at most `k`), (`n`  $\geq 0$ , `k`  $\geq 0$ ).

`SelfConjugatePartitions(n::RngIntElt) -> SeqEnum`

The unrestricted self-conjugate partitions of `n` (`n`  $\geq 0$ ).

`NumberOfSelfConjugatePartitions(n::RngIntElt) -> RngIntElt`

The number of unrestricted self-conjugate partitions of the non-negative integer `n`.

`SelfConjugateEndoskeleton(pa::[RngIntElt]) -> SeqEnum`

Computes the largest self-conjugate partition contained within the partition `pa`.

`SelfConjugateExoskeleton(pa::[RngIntElt]) -> SeqEnum`

Computes the smallest self-conjugate partition containing the partition `pa`.

## 1.5 Iterator for partitions

To construct all partitions of `n`, Magma has the in-built command `Partitions(n)`. This is very space-intensive for `n`  $\geq 100$ , so an iterator is required. We also include a function that computes the partition that has position `m` in the lexicographic ordering on partitions.

`NextPartition(pa::SeqEnum[RngIntElt],n::RngIntElt) -> SeqEnum`

Given a partition `pa` of size `n` (where `n` is specified to speed up calculations slightly), returns the next partition in the lexicographic ordering on partitions. If  $(1^n)$  is given as input, it returns  $(n)$ . Note that no checking is done as to whether the input is a partition with no trailing zeros, to maintain speed.

`NextPartition(~pa::SeqEnum[RngIntElt],n::RngIntElt)`

Given a partition `pa` of size `n` (where `n` is specified to speed up calculations slightly), destructively returns the next partition in the lexicographic ordering on partitions. If  $(1^n)$  is given as input, it returns  $(n)$ . Note that no checking is done as to whether the input is a partition with no trailing zeros, to maintain speed.

`NextPartition(pa::SeqEnum[RngIntElt]) -> SeqEnum`

Given a partition `pa` of length `n`, returns the next partition in the lexicographic ordering on partitions. If  $(1^n)$  is given as input, it returns  $(n)$ .

`NextPartition(~pa::SeqEnum[RngIntElt])`

Given a partition `pa` of length `n`, destructively returns the next partition in the lexicographic ordering on partitions. If  $(1^n)$  is given as input, it returns  $(n)$ .

`IndexToPartition(n::RngIntElt,m::RngIntElt) -> SeqEnum`

Given a non-negative integer  $n$  and a positive integer  $m$ , returns the  $m$ th partition of size  $n$  in the lexicographic ordering on partitions, so the  $m$ th entry in the sequence `Partitions(n)`.

`IndexToPartition(P::SeqEnum[RngIntElt]) -> RngIntElt`

Returns the index of the partition with respect to lexicographical ordering among partitions of the same size. (One is the first index by default, can be changed with the parameter `StartAtIndex`.) This is much faster than the inbuilt Magma command `IndexOfPartition` for larger partitions. Note that the Magma command starts counting at 0 whereas this function counts at 1, so it inverts the `IndexToPartition` function.

## 1.6 Hooks, $\beta$ -sets, etc.

This section covers extra commands regarding moving between  $\beta$ -sets and partitions, and other things associated to  $\beta$ -sets.

`IsBetaSet(X::SetEnum[RngIntElt]) -> BoolElt,SeqEnum`

Returns true and the corresponding partition if  $X$  is a beta set, and false otherwise.

`PartitionToBetaSet(pa::SeqEnum[RngIntElt]) -> SetEnum`

Returns the corresponding 'standard' beta-set to the partition  $pa$ . This is the beta-set with no 0.

`BetaSetToPartition(X::SetEnum[RngIntElt]) -> SeqEnum`

Returns the partition corresponding to the beta-set  $X$ .

`StandardBetaSet(X::SetEnum[RngIntElt]) -> SetEnum`

Returns the standard beta-set equivalent to  $X$ .

`AreEquivalent(X::SetEnum[RngIntElt],Y::SetEnum[RngIntElt]) -> BoolElt,SetEnum`

Returns true if the beta-sets  $X$  and  $Y$  are equivalent, and if so the standard beta-set equivalent to both of them.

`ConjugateBetaSet(X::SetEnum[RngIntElt]) -> SetEnum`

The standard beta-set corresponding to the conjugate partition of the partition corresponding to the beta-set  $X$ .

`HookLengths(pa::SeqEnum[RngIntElt]) -> SetMulti`

Returns the multiset of hook lengths of the partition  $pa$ .

`PrintAbacus(pa::SeqEnum[RngIntElt],t::RngIntElt) -> MonStgElt`

Prints the  $t$ -abacus corresponding to the partition  $pa$ .

`PrintAbacus(X::SetEnum[RngIntElt],t::RngIntElt) -> MonStgElt`

Prints the t-abacus corresponding to the beta-set X of first-column hook lengths.

## 1.7 Conjugacy classes

`NumberOfSymmetricConjugacyClassSizes(n::RngIntElt) -> RngIntElt`

Returns the cardinality of the set of conjugacy class sizes of the symmetric group of degree n. For n up to 100 this is returned from a lookup table. Otherwise the result is calculated, which can take some time.

## Chapter 2

# Character degrees and their multiplicities

One of the more interesting aspects of symmetric group representation theory is how certain questions, which are very easy for groups of Lie type, are incredibly difficult for symmetric groups, and vice versa. While it is fairly easy to understand minimal degrees of symmetric group representations, second and third minimal, and even higher, for groups of Lie type this is a difficult problem that has mostly been solved now.

On the other hand, it's generally not so bad to describe what characters of large degree look like. Asymptotically they are the Steinberg, and Deligne–Lusztig theory gives us a relatively satisfactory answer.

For symmetric groups things are much harder in some sense.

### 2.1 Maximal character degrees

These functions use a lookup table up to  $n = 150$ . Above that they construct the answer, which is quite slow and uses a large amount of memory. This will fail if your computer has less than 5TB of RAM.

`MaximalSymmetricCharacterDegree(n::RngIntElt) -> RngIntElt, SetEnum`

Returns the largest degree of an irreducible character of the symmetric group of degree  $n$ . The first output is the degree, the second is the set of partitions corresponding to the irreducible characters of that degree. For  $n$  at most 150 this is returned from a lookup table. Otherwise the result is calculated, which will take a long time and definitely fail if your computer has less than 5TB of RAM.

`SecondMaximalSymmetricCharacterDegree(n::RngIntElt) -> RngIntElt, SetEnum`

Returns the second largest degree of an irreducible character of the symmetric group of degree  $n$ . The first output is the degree, the second is the set of partitions corresponding to the irreducible characters of that degree. For  $n$  at most 150 this is returned from a lookup table. Otherwise the result is calculated, which will take a long time and definitely fail if your computer has less than 5TB of RAM.

`ThirdMaximalSymmetricCharacterDegree(n::RngIntElt) -> RngIntElt, SetEnum`

Returns the third largest degree of an irreducible character of the symmetric group of degree  $n$ . The first output is the degree, the second is the set of partitions corresponding to the irreducible characters of that

degree. For  $n$  at most 150 this is returned from a lookup table. Otherwise the result is calculated, which will take a long time and definitely fail if your computer has less than 5TB of RAM.

## 2.2 Multiplicities of character degrees

These functions also use a lookup table up to  $n = 129$ . Above that there are hard limits in Magma about the size of constructible sets that make things challenging, and the values of the functions below have not been calculated.

`MaximumMultiplicityOfSymmetricCharacterDegree(n::RngIntElt) -> RngIntElt`

Returns the largest multiplicity of an irreducible character degree for the symmetric group of degree  $n$ . For low values of  $n$  this is returned from a lookup table. Above that we start hitting the limits of how big a set Magma is capable of constructing, so values above that have not been found.

`NumberOfIrreducibleSymmetricCharacterDegrees(n::RngIntElt) -> RngIntElt`

Returns the cardinality of the set of irreducible character degrees of the symmetric group of degree  $n$ . For  $n$  up to 129 this is returned from a lookup table. Above that we start hitting the limits of how big a set Magma is capable of constructing, so values above 129 have not yet been found.

`AverageMultiplicityOfSymmetricCharacterDegree(n::RngIntElt:AsRational) -> .`

Returns the average multiplicity of an irreducible character degree of the symmetric group of degree  $n$ . If the parameter `AsRational` is set to be true, a rational number is returned. Otherwise a real number is returned. For  $n$  up to 129 this is returned from a lookup table. Above 129 we start hitting the limits of how big a set Magma is capable of constructing, so values above 129 have not yet been found.

`MaximumMultiplicityOfSymmetricCharacterDegreeExceeds(n::RngIntElt,d::RngIntElt:IgnoreSelfConjugatePartitions) -> BoolElt`

Returns true if the maximum multiplicity of an irreducible character degree of the symmetric group of degree  $n$  exceeds  $d$ . This is checked with a lookup table for  $n$  at most 129 and by constructing enough character degrees to decide on the truth of the question if  $n$  is larger.

If the parameter `IgnoreSelfConjugatePartitions`, default false, is set to true, only partitions that are not self-conjugate are considered, for applications to alternating groups.

## 2.3 $\infty$ -partitions and partition clusters

This section deals with  $\infty$ -partitions and clusters of partitions. These are taken from the paper *Symmetric group character degrees and hook numbers* from 2008, and are used to find collections of irreducible characters of  $S_n$  that all have the same hook lengths (clusters of partitions). We will not define the terms in this section, as you will probably not need this unless you are familiar with that paper.

We give a new type, `InfPart`, which has a partition and a period as its inputs.

### 2.3.1 General commands

`InfinityPartition(pa::SeqEnum[RngIntElt],p::RngIntElt) -> InfPart`

Given a partition  $pa$  of at most  $p$  parts, and an integer  $p$ , construct the corresponding infinity-partition.

`MissingHookLengths(X::InfPart) -> SetMulti`

The missing hook lengths of the infinity-partition  $X$ .

`SplinteredInfinityPartition(X::InfPart) -> InfPart`

The splintered infinity-partition corresponding to  $X$ .

`IsCluster(X::SetEnum[InfPart]) -> BoolElt`

`IsCluster(X::SeqEnum[InfPart]) -> BoolElt`

Returns true if the set  $X$  of infinity-partitions all have the same missing hook lengths.

`IsCluster(X::SeqEnum[SeqEnum]) -> BoolElt`

`IsCluster(X::SeqEnum[SeqEnum]) -> BoolElt`

Checks whether all partitions in  $X$  have the same hook lengths.

`IsPeriodicCluster(X::SeqEnum[SeqEnum[RngIntElt]]) -> BoolElt,SetEnum`

`IsPeriodicCluster(X::SetEnum[SeqEnum[RngIntElt]]) -> BoolElt,SetEnum`

Returns whether  $X$  is a cluster of partitions, and the set of integers  $p$  for which  $X$  forms a periodic cluster of period  $p$ . If the cluster is not periodic, it will return false.

`PeriodicClusterGenerator(X::SetEnum[SeqEnum[RngIntElt]],p::RngIntElt) -> SetEnum`

Given a periodic cluster  $X$  with period  $p$ , returns the smallest periodic cluster in the same sequence as  $X$ , with the condition that the conjugate partitions of the elements in the cluster are distinct from the cluster. (The period must be specified as clusters may have more than one period.)

`PeriodicClusterExtension(X::SetEnum[SeqEnum[RngIntElt]],p::RngIntElt,n::RngIntElt) -> SetEnum`

Given a periodic cluster  $X$  with period  $p$ , returns the periodic cluster obtained by extending this cluster by  $n$ . Note that while  $n$  may be negative, it cannot reduce the size of the cluster below that of the generator of the periodic cluster.

`DetermineClustersOfPartitions(n::RngIntElt) -> SeqEnum,SeqEnum`

Determines all clusters among the partitions of of size  $n$ . The function returns the clusters of partitions, and also the hook lengths of each cluster. The function `DetermineLargeClustersOfPartitions` should be used if one wants just the clusters of order at least 3, as it is faster.

`DetermineLargeClustersOfPartitions(n::RngIntElt) -> SeqEnum`

Determines all clusters of size at least 3 among the partitions of of size  $n$ . The function returns the clusters of partitions, and also the hook lengths of each cluster. This method is faster than `DetermineClustersOfPartitions`.

`MatchInfinityPartitionsToClusters(X::SeqEnum[SetEnum[InfPart]],R::SeqEnum[SetEnum[SeqEnum]])  
-> SeqEnum[SetEnum[SeqEnum]]`

Given a collection  $X$  of clusters of infinity-partitions and a set  $R$  of clusters of partitions, finds all periodic

clusters with infinity-partition from  $X$  and remainder from  $R$ . At the moment, all clusters in  $X$  and  $R$  should have cardinality 4 for this to work, as it is optimized to find periodic clusters of cardinality 8 (when taken with their conjugates).

`EnvelopingPartition(pa::SeqEnum[RngIntElt]) -> SeqEnum`

Returns the enveloping partition corresponding to the partition `pa`. If `pa` and `pa2` have the same hook lengths then so do their enveloping partitions. Furthermore, they form a periodic cluster. This is the central construction in the 2008 paper of Craven.

### 2.3.2 Commands to access databases

`InfinityPartitionClusters(p::RngIntElt) -> SeqEnum`

The known set of infinity-partition clusters of cardinality 4, small partition size and period at most 10. If  $p > 10$  then no clusters are stored. If  $p < 7$  then there are no clusters.

`PeriodicPartitionClusters(p::RngIntElt) -> SeqEnum`

The known set of periodic partition clusters of cardinality 4 (8 with conjugates), small partition size and period at most 10. If  $p > 10$  then no clusters are stored. If  $p < 7$  then there are no clusters.

`PartitionClusters() -> SeqEnum`

Returns all clusters of size greater than 2 for partitions of size at most 60.

`LargePartitionClusters(n::RngIntElt) -> SeqEnum`

Returns all clusters of size greater than 2 for partitions of size  $n$  for  $n$  between 61 and 90.

## 2.4 Characters for $GL_n(q)$ and $GU_n(q)$

This section gives some functions for computing the generic degrees of unipotent characters for  $GL_n(q)$  and  $GU_n(q)$ , using the standard formula. They are included here as the degrees are closely related to those of the symmetric group, and use the hook formula.

`LusztigaFunction(pa::[RngIntElt]) -> RngIntElt`

Returns the Lusztig  $a$ -function associated to the partition `pa`, i.e., the sum over  $i$  of  $(i-1)$  times the size of the  $i$ th part of `pa`.

`LusztigAFunction(pa::[RngIntElt]) -> RngIntElt`

Returns the Lusztig  $A$ -function associated to the partition `pa`, i.e., the degree of the generic degree of the unipotent character, so the sum of the Lusztig  $a$ -function and  $n + 1$  choose 2 minus the sum of the hook lengths of `pa`.

`GLGenericDegree(pa::[RngIntElt]) -> RngUPolElt`

Computes the generic degree of the unipotent character of  $GL_n(q)$  associated to the partition `pa`.

`GUGenericDegree(pa::[RngIntElt]) -> RngUPolElt`

Computes the generic degree of the unipotent character of  $\mathrm{GU}_n(q)$  associated to the partition  $\mathbf{pa}$ .

## Chapter 3

# Restrictions of characters of Sylow subgroups

These commands concern restricting characters to Sylow  $p$ -subgroups  $P$  of symmetric groups, and calculating their inner products with linear characters of the symmetric groups. Since characters of  $S_n$  are constant on cycle types, when restricting to a Sylow  $p$ -subgroup we only need understand the values of the character on cycle types all of whose parts are powers of  $p$ . We then need to understand the distribution of those cycle types among the conjugacy classes of  $P$ . If, however, we consider linear characters only, it suffices to understand the cycle type structure among the cosets of the derived subgroup  $P'$  of  $P$ , which is a soluble problem. The matrix of this distribution has been computed for  $n = 4, 8, 16, 32, 64, 128$ , so calculations can be made for these  $n$  when  $p = 2$ . For  $p$  odd this can in theory be done, but choices about the linear characters, their labelling and so on need to be made, and I have not done so at this time. (For  $p$  odd, the restrictions of characters of  $S_n$  cannot be used to distinguish between linear characters of  $P$ . One can see this since characters of  $P$  have  $p$ th roots of unity and characters of  $S_n$  are integer-valued. Thus it seems reasonable to bundle together all Galois orbits of linear characters for  $P$ .)

Some of the commands below take the prime  $p$  as a parameter as well, because they have been written in a characteristic-free manner.

```
PartitionToGroupElement(pa::SeqEnum[RngIntElt]) -> GrpPermElt
```

A permutation of a symmetric group with cycle type `pa`. Although the name suggests that `pa` must be a partition, any composition will work.

```
SymmetricCharacterValue(pa::SeqEnum[RngIntElt], pe::SeqEnum[RngIntElt]) -> RngIntElt
```

Returns the irreducible character value for the character labelled by the partition `pa` on a permutation of a symmetric group with cycle type the composition `pe`.

```
SymmetricCharacterValues(pa::SeqEnum[RngIntElt], cy::SeqEnum[SeqEnum[RngIntElt]]) -> SeqEnum
```

The values of the irreducible character labelled by the partition `pa` evaluated at the cycle types given by `cy`. Note that `cy` is a list of partitions/compositions, and not a list of group elements.

```
SymmetricSylowCycleTypes(n::RngIntElt, p::RngIntElt) -> SeqEnum
```

A list of all possible cycle types of elements in a Sylow  $p$ -subgroup of a symmetric group of degree  $n$ .

`SymmetricSylow2LinearCharacters(n::RngIntElt) -> Mtrx`

The linear characters of a Sylow 2-subgroup of the symmetric group of degree  $n$ , given as a (square) matrix. Note that  $n$  must be a power of 2. This function has a certain labelling of the rows and columns. The labelling of the columns is based on the structure of the Sylow subgroup of the symmetric group, and the labelling of the rows is arbitrary.

`SymmetricCharacterSylowRestriction(pa::SeqEnum[RngIntElt],p::RngIntElt) -> SeqEnum`

Returns the restriction of the irreducible character labelled by the partition  $pa$  to a Sylow  $p$ -subgroup of the symmetric group. The ordering on the elements of a Sylow  $p$ -subgroup of the symmetric group is given by the function `SymmetricSylowCycleTypes`. For hook partitions restricted to the Sylow  $p$ -subgroup, use the function `SymmetricCharacterHookRestrictions`.

`SymmetricCharacterHookRestrictions(n::RngIntElt,p::RngIntElt) -> SeqEnum`

Computes (quickly) the restrictions of characters associated to all hook partitions to a Sylow  $p$ -subgroup of the symmetric group of degree  $n$ .

`SymmetricSylowConjugateCharacter(ch::SeqEnum[RngIntElt],n::RngIntElt) -> SeqEnum`

Given a character of a symmetric group of degree  $n$  restricted to a Sylow 2-subgroup, returns the conjugate character, i.e., the tensor product of  $ch$  with the sign character. (This function is not needed if  $p$  is odd, as there are no conjugate characters of a Sylow  $p$ -subgroup.)

`SymmetricSylowRestrictionInnerProducts(ch::SeqEnum[RngIntElt],n::RngIntElt) -> SeqEnum`

Returns the list of inner products of the restricted character  $ch$  of the symmetric group of degree  $n$  with the linear characters according to the labelling by hook partitions. This method currently only works for  $n$  in  $\{4, 8, 16, 32, 64, 128\}$ .

`SymmetricSylowRestrictionInnerProducts(X::SeqEnum[SeqEnum[RngIntElt]],n::RngIntElt) -> SeqEnum`

Returns the list of inner products of the collection  $X$  of restricted characters of the symmetric group of degree  $n$  with the linear characters according to the labelling by hook partitions. This method currently only works for  $n$  in  $\{4, 8, 16, 32, 64, 128\}$ .

## Chapter 4

# Changes since original

### Changes in V1.4

- Maximum multiplicities and character degree set lookup tables increased to 129.
- Increased `LargePartitionClusters` up to `n` at most 90.

### Changes in V1.3

- New function `PartitionToIndex`, which is much faster than the Magma inbuilt function `IndexOfPartition` for larger partitions, over around size 80.
- Increased `LargePartitionClusters` up to `n` at most 87.
- Maximal character degree values increased to 150.

### Changes in V1.2

- Fixed a bug in `InfinityPartition` constructor.
- Added commands `PrintReducedFormPartition`, `NumberOfPartitionsWithAtMostParts`, `NumberOfPartitionsWithExactlyParts`, `SelfConjugateEndoskeleton`, `SelfConjugateExoskeleton`, `IndexToPartition`, `NumberOfSymmetricConjugacyClassSizes` `EnvelopingPartition`, `LargePartitionClusters`, `DetermineLargeClustersOfPartitions`, `LusztigaFunction`, `LusztigAFunction`, `GLGenericDegree` and `GUGenericDegree`.
- Functions in Sylow restrictions section upgraded to deal with `n = 128`.
- Maximum multiplicities and character degree set lookup tables increased to 115.
- Maximal character degree values increased to 135.

### Changes in V1.1

- Improved some help wording.
